# Supplementary material for: VideoFACT: Detecting Video Forgeries Using Attention, Scene Context, and Forensic Traces
Source: arXiv:2211.15775 source file (2023-03-10)
Supplement: Supplementary file 1 [file 205_training_details.tex]

\section{Training Details}
\label{appendix:training_details}
